# Supplementary material for: Surface microlenses for much more efficient photodegradation in water treatment
Source: arXiv:2204.01842 source file (2022-03-31)
Supplement: Supplementary file 1 [file Supplementary_information.pdf]

Supporting Information

# Surface microlenses for much more efficient photodegradation in water treatment

*Qiuyun Lu*[a], *Qiwei Xu*[b], *Jia Meng*[a], *Zuo Tong How*[c], *Pamela Chelme-Ayala*[c], *Xihua Wang*[b,*], *Mohamed Gamal El-Din*[c,*] *and Xuehua Zhang* [a,*]

[a] Department of Chemical and Materials Engineering, University of Alberta, 9211 116 Street NW, Edmonton, T6G 1H9, Canada

[b] Department of Electrical and Computer Engineering, University of Alberta, 9211 116 Street NW, Edmonton, T6G 1H9, Canada

[c] Department of Civil and Environmental Engineering, University of Alberta, 9211 116 Street NW, Edmonton, T6G 1H9, Canada

*E-mails: mailto:xihua@ualberta.ca (X. Wang); mgamalel-din@ualberta.ca (M.G. El-Din); mailto:xuehua.zhang@ualberta.ca (X. Zhang)

**Electron spin resonance (ESR) detection**

The electron spin resonance (ESR) technology is utilized to verify if free radicals play an important role in the photodegradation process. The ESR spectrum of samples that are irradiated for 30 min in presence of a spin trap is displayed in Figure S2. There are no characteristic signals of free radicals, such as hydroxyl radicals and superoxide radicals, detected in samples after light treatment no matter surface MLs are used or not. The ESR spectrum indicates that the above-mentioned free radicals do not participate in the photodegradation in the first 30 min of photodegradation. The results also prove that the use of surface MLs does not cause the formation of free radicals.

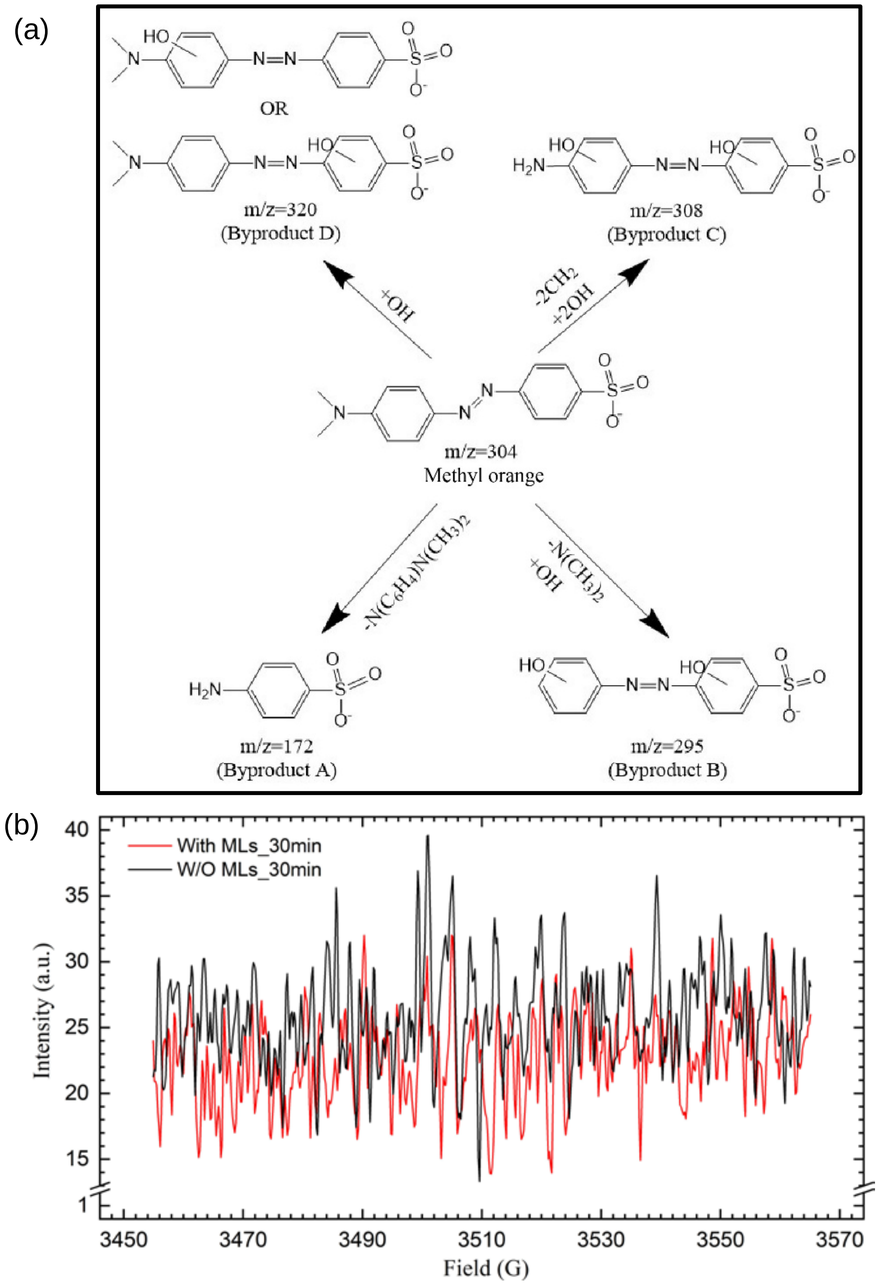


**Figure S1.** (a) The possible cleavage position (m/z is the mass-to-charge ratio of certain species. Byproduct A: m/z=172.0059, byproduct B: m/z=294.9452, byproduct C: m/z=308.0758, byproduct D: m/z=320.0653) in a MO molecule in the photodegradation. (b) The electron spin resonance spectrum of methyl orange (MO) solution after the light treatment without MLs and with MLs for 30 min, using 50 mM DMPO as the spin trap.

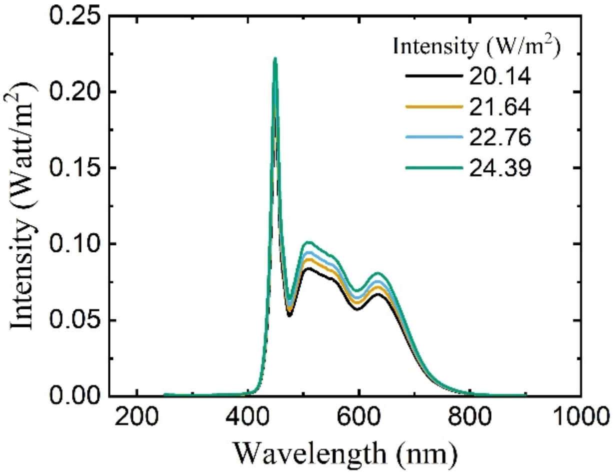


**Figure S2.** Light spectrum of the light resource (wavelength: 300-900 nm) with different intensities (20.12, 21.64, 22.76, and 24.39 W/$m^2$).

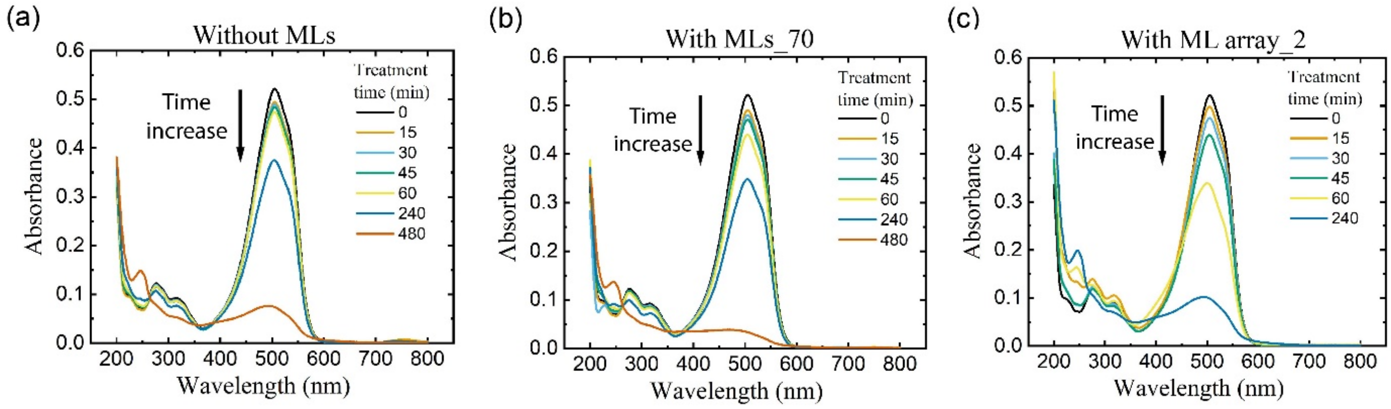


**Figure S3.** The UV-vis absorbance curves of MO solution after irradiation (a) without MLs, (b) with MLs_70, and (c) with ML array_2 as the light treatment time increased. The concentration of MO solution was 5 mg/L, with pH=3.0. The MO solution was degassed for 15 min before light treatment, and the light intensity was 21.64 W/$m^2$.

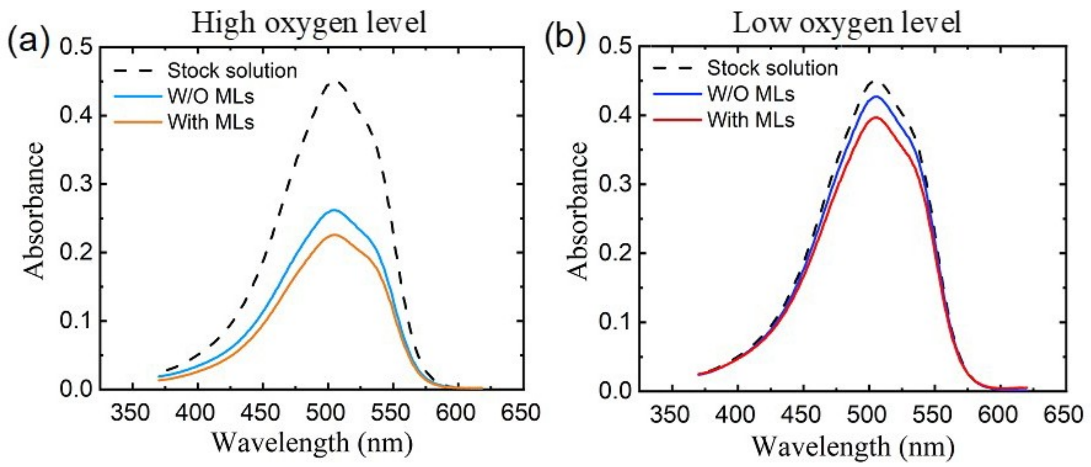


**Figure S4.** Absorbance curves of MO solution at (a) high oxygen level (no degassing step before treatment) and (b) low oxygen level (degassing for 15 min before light treatment). The MO solution (initial MO concentration: 5 mg/L, pH value: 3.0) was irradiated for 1 hour. The black dashed lines represent the solution before treatment, while the colorful solid lines show the solution after treatment without (W/O) and with MLs.

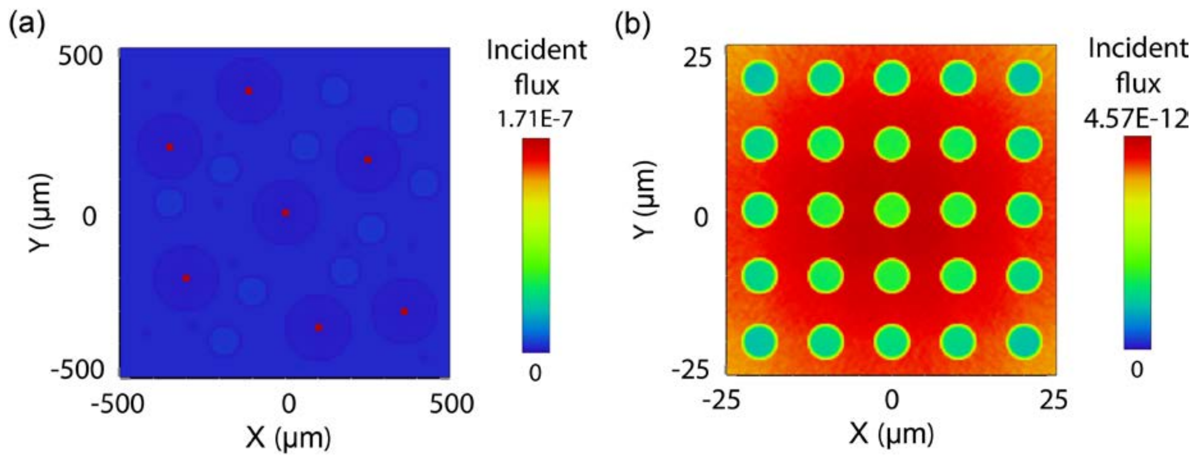


**Figure S5.** Top-view intensity profiles of (a) random MLs on homogeneous hydrophobic substrate and (b) ML array at the depth of 224 μm.

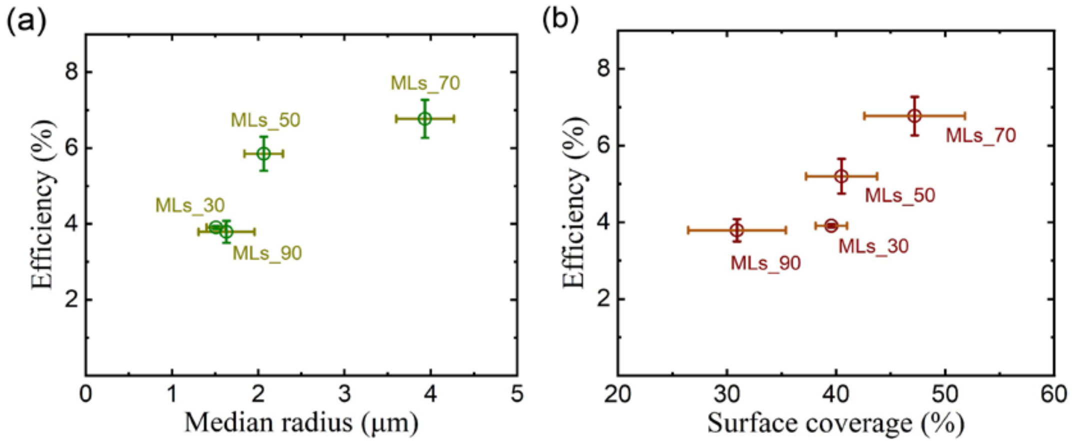


**Figure S6.** The photodegradation efficiency of MO solution after irradiation of 30 min with (a) surface coverage and (b) median lateral radius of random MLs.
